# Supplementary material for: Ab initio studies of the ground and first excited states of the Sr-H$_2$ and Yb-H$_2$ complexes
Source: arXiv:1807.05228 source file (2019-07-12)
Supplement: Supplementary file 1 [file Supplementary-material.pdf]

Supplementary material for:

# *Ab initio* studies of the ground and first excited states of the Sr–$H_2$ and Yb–$H_2$ complexes

Hubert Cybulski*

*Institute of Physics, Faculty of Physics, Astronomy and Informatics, Nicolaus Copernicus University in Torun, Grudziadzka 5, 87-100 Torun, Poland*

*hubert@fizyka.umk.pl, hcybulski@gmail.com

## I. Analytical fits of the ground-state IPESs

The *ab initio* interaction energies for both the ground-state IPESs were fitted using the analytical function $V(R,\theta)$ originally suggested by Bukowski *et al.* [1] and successfully adopted in the fitting of interaction energies in similar systems [2, 3].

The function $V(R,\theta)$ is written as the sum of a short range term $V_{\mathrm{sh}}$ and an asymptotic term $V_{\mathrm{as}}$:

$$V(R,\theta) = V_{\mathrm{sh}}(R,\theta) + V_{\mathrm{as}}(R,\theta). \tag{1}$$

The short range term is

$$V_{\mathrm{sh}}(R,\theta) = G(R,\theta)e^{D(\theta)-B(\theta)R}, \tag{2}$$

where the angular parts of $B(\theta)$ and $G(R,\theta)$ are given by the following expansions in the Legendre polynomials

$$B(\theta) = \sum_{l=0}^{l_{\mathrm{max}}} b_l P_l^0(\cos\theta), \tag{3}$$

$$D(\theta) = \sum_{l=0}^{l_{\mathrm{max}}} d_l P_l^0(\cos\theta), \tag{4}$$

$$G(R,\theta) = \sum_{l=0}^{l_{\mathrm{max}}} \left( \sum_{n=0}^{n_{\mathrm{max}}} g_{(n,l)} R^n \right) P_l^0(cos\theta). \tag{5}$$

Because of the symmetry of the systems only even values of $l$ were employed.

The asymptotic term is represented by

$$V_{\mathrm{as}}(R,\theta) = \sum_{n=6,8,10} f_n(B(\theta)R) \left[ \sum_{k=0,2} \left( \frac{C_n^k}{R^n} \right) P_k^0(\cos\theta) \right] \tag{6}$$

where $f_n$ is the $n$-th Tang-Toennies damping function [4]:

$$f_n(B(\theta)R) = 1 - e^{-B(\theta)R} \sum_{k=0}^{n} \frac{(B(\theta)R)^k}{k!} \tag{7}$$

Each fitting process was started by employing all the *ab initio* points corresponding to $R \geq 9$ Å and fitting the long-range constants $C_n^k$ assuming no damping. Subsequently, the $C_n^k$ values were frozen and the remaining parameters were fitted to all the *ab initio* data points with energies lower than 200 cm$^{-1}$.

The optimised parameters of the fitted functions are collected in Table 1. For the Sr-$H_2$ (Yb-$H_2$) IPESs we obtain root-mean-square errors lower than $1.53 \cdot 10^{-2}$ cm$^{-1}$ ($5.19 \cdot 10^{-3}$ cm$^{-1}$). The maximum errors for each IPES are lower than $8.43 \cdot 10^{-2}$ cm$^{-1}$ ($1.30 \cdot 10^{-2}$ cm$^{-1}$) for the Sr-$H_2$ (Yb-$H_2$) system.

Fortran subroutines for generating the potentials are attached to this Supplementary Material.

Table 1: The optimised parameters of the fitted functions for the ground state of the Sr-$H_2$ and Yb-$H_2$ complexes. Not all digits listed here are significant: the extra digits are given for consistency with the programmed expressions. The analytic functions require distances $R$ in angstroms, angles in radians and return potential values in $cm^{-1}$

| Parameter | Sr-$H_2$ | Yb-$H_2$ |
|---|---|---|
| $b_0$ | 2.325786071272089 | 2.192805237055535 |
| $b_2$ | -5.055422539960337·$10^{-2}$ | 1.668683618864231·$10^{-1}$ |
| | | |
| $d_0$ | -4.661539782516745·$10^{-1}$ | 1.939281629570284 |
| $d_2$ | 6.149097369325915·$10^{-1}$ | 8.679533674890181·$10^{-1}$ |
| | | |
| $g_{(0,0)}$ | 3.287584515676756·$10^{7}$ | 6.217483880907111·$10^{5}$ |
| $g_{(0,2)}$ | -1.072554993152140·$10^{7}$ | 1.340288584839195·$10^{6}$ |
| $g_{(0,4)}$ | 9.329507229174780·$10^{6}$ | 4.368433819885250·$10^{4}$ |
| $g_{(0,6)}$ | — | -2.017385985607475·$10^{2}$ |
| | | |
| $g_{(1,0)}$ | -3.089986564494018·$10^{7}$ | -9.036995015662524·$10^{5}$ |
| $g_{(1,2)}$ | 1.063730247655489·$10^{7}$ | -1.289974019270727·$10^{6}$ |
| $g_{(1,4)}$ | -6.902252987889808·$10^{6}$ | -1.917606989930055·$10^{4}$ |
| $g_{(1,6)}$ | -1.498563321536317·$10^{4}$ | — |
| | | |
| $g_{(2,0)}$ | 1.098666987790165·$10^{7}$ | 5.410525311925033·$10^{5}$ |
| $g_{(2,2)}$ | -3.624989303067407·$10^{6}$ | 4.559472810722237·$10^{5}$ |
| $g_{(2,4)}$ | 1.741609332521859·$10^{6}$ | 1.947540324062861·$10^{3}$ |
| | | |
| $g_{(3,0)}$ | -1.371527457032413·$10^{6}$ | -1.270440714314889·$10^{5}$ |
| $g_{(3,2)}$ | 3.077529564533590·$10^{5}$ | -7.713667622882128·$10^{4}$ |
| $g_{(3,4)}$ | -1.354662511845866·$10^{5}$ | — |
| | | |
| $g_{(4,0)}$ | 5.449532347534497·$10^{4}$ | 1.362684384049058·$10^{4}$ |
| $g_{(4,2)}$ | — | 6.708328463113382·$10^{3}$ |
| | | |
| $g_{(5,0)}$ | — | -5.610364527541666·$10^{2}$ |
| $g_{(5,2)}$ | — | -2.387322015154814·$10^{2}$ |
| | | |
| $C_6^0$ | -7.120738688734989·$10^{5}$ | -7.008819510639583·$10^{5}$ |
| $C_6^2$ | -9.295748817247465·$10^{4}$ | -4.651950404335265·$10^{4}$ |
| | | |
| $C_8^0$ | -1.548729223914000·$10^{7}$ | 1.095495734547660·$10^{7}$ |
| $C_8^2$ | 4.352040259284884·$10^{6}$ | -3.487259066878202·$10^{6}$ |
| | | |
| $C_{10}^0$ | -2.781181859819762·$10^{8}$ | -1.188235596326569·$10^{9}$ |
| $C_{10}^2$ | -4.689999658659733·$10^{8}$ | — |

## II. Complete tables for the basis set studies

Table 2: The CCSD(T) interaction energy values (in $cm^{-1}$) for the ground state of the Yb-$H_2$ complex in the collinear geometry. The intermolecular distance values $R$ are given in angstroms. In all the calculations the 332211 midbond function set was used. See inside the article for more details regarding the used basis functions (bfs)

| | | | | | | | |
|---|---|---|---|---|---|---|---|
| Yb | | | | | | | |
| PP | ECP28MWB | ECP28MWB | ECP28MWB | ECP28MWB | ECP28MWB | ECP28MWB | |
| Basis set | ECP28MWB-ANO | ECP28MWB-ANO | ECP28MWB-ANO | ECP28MWB-ANO | ECP28MWB-ANO | ECP28MWB-ANO | uANO-RCC |
| Additional bfs | | 1 even | $h$ + 1 even | $h$, $i$ + 1 even | 2 even | 1 even | |
| H | | | | | | | |
| Basis set | aDZ | aDZ | aDZ | aDZ | aDZ | aTZ | uANO-RCC |
| Number of bfs | 178 | 203 | 258 | 297 | 228 | 231 | 441 |
| R | Interaction energy | | | | | | |
| 4.20 | 69.91 | 66.88 | 65.80 | 65.68 | 67.19 | 67.74 | 51.36 |
| 4.40 | 20.94 | 19.05 | 18.25 | 18.18 | 19.34 | 19.43 | 8.21 |
| 4.60 | -6.90 | -7.88 | -8.50 | -8.57 | -7.53 | -8.21 | -15.53 |
| 4.80 | -21.17 | -21.56 | -22.06 | -22.15 | -21.16 | -22.56 | -27.12 |
| 5.00 | -27.01 | -27.11 | -27.49 | -27.64 | -26.75 | -28.65 | -31.38 |
| 5.20 | -28.00 | -27.99 | -28.22 | -28.40 | -27.80 | -29.81 | -31.45 |
| 5.40 | -26.72 | -26.62 | -26.72 | -26.84 | -26.67 | -28.21 | -29.32 |
| 5.60 | -24.61 | -24.39 | -24.43 | -24.49 | -24.59 | -25.39 | -26.20 |
| 5.80 | -22.10 | -21.81 | -21.84 | -21.87 | -22.02 | -22.30 | -22.78 |
| 6.00 | -19.36 | -19.08 | -19.11 | -19.14 | -19.24 | -19.32 | -19.48 |

Table 3: The CCSD(T) interaction energy values (in $cm^{-1}$) for the ground state of the Yb-$H_2$ complex in the collinear geometry. The intermolecular distance values $R$ are given in angstroms. In all the calculations the 332211 midbond function set was used. See inside the article for more details regarding the used basis functions (bfs). $CBS_{X/Y}$ stands for the CBS limit calculated with the XZ-DK and YZ-DK basis sets

| Basis set | DZ-DK | DZ-DK | DZ-DK | TZ-DK | uTZ-DK | TZ-DK | TZ-DK | TZ-DK | QZ-DK | QZ-DK | QZ-DK | uANO-RCC | $CBS_{D/T}$ | $CBS_{T/Q}$ |
|---|---|---|---|---|---|---|---|---|---|---|---|---|---|---|
| Additional bfs | | 1 even | 2 even | | | 1 even | 2 even | 3 even | | 1 even | 2 even | | | |
| Number of bfs | 150 | 183 | 216 | 229 | 385 | 283 | 337 | 391 | 330 | 411 | 492 | 441 | 150/229 | 229/330 |
| R | Interaction energy | | | | | | | | | | | | | |
| 4.20 | 65.80 | 55.09 | 52.77 | 59.41 | 58.56 | 53.06 | 52.09 | 51.78 | 53.75 | 50.52 | 50.11 | 51.36 | 55.23 | 51.83 |
| 4.40 | 20.59 | 9.64 | 7.98 | 15.20 | 14.45 | 9.43 | 8.73 | 8.51 | 10.53 | 7.64 | 7.35 | 8.21 | 11.68 | 8.74 |
| 4.60 | -4.75 | -15.93 | -16.80 | -9.52 | -10.07 | -14.75 | -15.20 | -15.36 | -13.31 | -15.91 | -16.13 | -15.53 | -12.54 | -14.92 |
| 4.80 | -17.57 | -28.29 | -28.78 | -21.95 | -22.29 | -26.62 | -26.92 | -27.02 | -25.03 | -27.35 | -27.51 | -27.12 | -24.63 | -26.45 |
| 5.00 | -22.87 | -32.42 | -33.07 | -26.94 | -27.11 | -31.06 | -31.27 | -31.33 | -29.46 | -31.52 | -31.63 | -31.38 | -29.38 | -30.70 |
| 5.20 | -23.92 | -32.02 | -33.04 | -27.66 | -27.70 | -31.26 | -31.41 | -31.43 | -29.72 | -31.54 | -31.62 | -31.45 | -29.85 | -30.80 |
| 5.40 | -22.73 | -29.51 | -30.73 | -26.10 | -26.03 | -29.20 | -29.32 | -29.32 | -27.78 | -29.37 | -29.43 | -29.32 | -28.02 | -28.71 |
| 5.60 | -20.51 | -26.19 | -27.38 | -23.48 | -23.37 | -26.13 | -26.21 | -26.22 | -24.80 | -26.22 | -26.27 | -26.20 | -25.11 | -25.55 |
| 5.80 | -17.94 | -22.69 | -23.74 | -20.50 | -20.36 | -22.77 | -22.82 | -22.82 | -21.64 | -22.80 | -22.84 | -22.78 | -21.86 | -22.33 |
| 6.00 | -15.38 | -19.34 | -20.22 | -17.57 | -17.44 | -19.49 | -19.52 | -19.53 | -18.49 | -19.49 | -19.53 | -19.48 | -18.68 | -19.07 |

Table 4: The CCSD(T) interaction energy values (in $cm^{-1}$) for the ground state of the Yb-$H_2$ complex in the T-shape geometry. The intermolecular distance values $R$ are given in angstroms. In all the calculations the 332211 midbond function set was used. See inside the article for more details regarding the used basis functions (bfs)

| Basis set | DZ-DK | TZ-DK | | | | QZ-DK | uANO-RCC |
|---|---|---|---|---|---|---|---|
| Additional bfs | | | 1 even | 2 even | 3 even | | |
| Number of bfs | 150 | 229 | 283 | 337 | 391 | 330 | 441 |
| R | Interaction energy | | | | | | |
| 5.20 | -14.56 | -18.57 | -21.28 | -21.57 | -21.67 | -20.50 | -21.39 |
| 5.40 | -14.89 | -18.56 | -20.98 | -21.21 | -21.27 | -20.17 | -21.03 |
| 5.60 | -13.96 | -17.25 | -19.42 | -19.60 | -19.65 | -18.63 | -19.44 |
| 5.80 | -12.45 | -15.36 | -17.31 | -17.46 | -17.49 | -16.54 | -17.31 |
| 6.00 | -10.77 | -13.29 | -15.07 | -15.19 | -15.22 | -14.33 | -15.06 |

## III. The calculated interaction energies for the Sr-$H_2$, Yb-$H_2$, Sr-He, and Yb-He complexes

Table 5: The calculated interaction energy values (in $cm^{-1}$) for the ground state of the Sr-$H_2$ complex. The intermolecular distance values $R$ are given in angstroms

| $\theta =$ R | 0.00 | 25.8737249750682 | 47.3758416495282 | 68.7082259546949 | 90.00 |
|---|---|---|---|---|---|
| 3.60 | 672.577 | 656.705 | 632.783 | 615.348 | 609.468 |
| 3.80 | 424.299 | 418.206 | 409.435 | 403.547 | 401.707 |
| 4.00 | 254.921 | 254.084 | 253.392 | 253.639 | 253.951 |
| 4.20 | 141.987 | 143.780 | 147.185 | 150.514 | 151.907 |
| 4.40 | 68.878 | 71.780 | 77.064 | 81.734 | 83.584 |
| 4.60 | 23.355 | 26.525 | 32.406 | 37.408 | 39.354 |
| 4.80 | -3.557 | -0.517 | 5.216 | 10.005 | 11.855 |
| 5.00 | -18.291 | -15.520 | -10.316 | -5.998 | -4.342 |
| 5.20 | -25.299 | -22.817 | -18.296 | -14.549 | -13.117 |
| 5.40 | -27.592 | -25.371 | -21.556 | -18.388 | -17.178 |
| 5.60 | -27.143 | -25.154 | -22.001 | -19.370 | -18.361 |
| 5.80 | -25.195 | -23.442 | -20.876 | -18.714 | -17.880 |
| 6.00 | -22.522 | -21.038 | -18.967 | -17.204 | -16.521 |
| 6.20 | -19.622 | -18.426 | -16.762 | -15.330 | -14.775 |
| 6.40 | -16.810 | -15.882 | -14.544 | -13.386 | -12.938 |
| 6.60 | -14.256 | -13.548 | -12.473 | -11.537 | -11.175 |
| 6.80 | -12.027 | -11.484 | -10.617 | -9.861 | -9.569 |
| 7.00 | -10.125 | -9.701 | -9.000 | -8.387 | -8.150 |
| 7.20 | -8.520 | -8.182 | -7.614 | -7.115 | -6.922 |
| 7.40 | -7.176 | -6.902 | -6.439 | -6.031 | -5.873 |
| 7.60 | -6.053 | -5.829 | -5.449 | -5.114 | -4.984 |
| 7.80 | -5.117 | -4.932 | -4.618 | -4.342 | -4.234 |
| 8.00 | -4.337 | -4.183 | -3.923 | -3.693 | -3.603 |
| 8.20 | -3.687 | -3.559 | -3.342 | -3.149 | -3.074 |
| 8.40 | -3.144 | -3.037 | -2.855 | -2.692 | -2.628 |
| 8.60 | -2.689 | -2.601 | -2.446 | -2.309 | -2.255 |
| 8.80 | -2.309 | -2.234 | -2.103 | -1.986 | -1.941 |
| 9.00 | -1.989 | -1.926 | -1.814 | -1.715 | -1.677 |
| 9.20 | -1.719 | -1.666 | -1.571 | -1.486 | -1.454 |
| 9.40 | -1.491 | -1.446 | -1.364 | -1.293 | -1.265 |
| 9.60 | -1.297 | -1.259 | -1.189 | -1.128 | -1.104 |
| 9.80 | -1.133 | -1.099 | -1.040 | -0.987 | -0.966 |
| 10.00 | -0.992 | -0.963 | -0.912 | -0.866 | -0.848 |
| 10.20 | -0.872 | -0.847 | -0.802 | -0.762 | -0.747 |
| 10.40 | -0.769 | -0.746 | -0.707 | -0.673 | -0.659 |

*Table 5 continues on next page...*

*Table 5 continues...*

| $\theta =$ R | 0.00 | 25.8737249750682 | 47.3758416495282 | 68.7082259546949 | 90.00 |
|---|---|---|---|---|---|
| 10.60 | -0.680 | -0.660 | -0.625 | -0.595 | -0.583 |
| 10.80 | -0.603 | -0.585 | -0.555 | -0.527 | -0.516 |
| 11.00 | -0.535 | -0.520 | -0.493 | -0.469 | -0.459 |
| 11.20 | -0.477 | -0.463 | -0.439 | -0.418 | -0.409 |
| 11.40 | -0.426 | -0.413 | -0.392 | -0.373 | -0.366 |
| 11.60 | -0.381 | -0.370 | -0.351 | -0.334 | -0.327 |
| 11.80 | -0.342 | -0.332 | -0.315 | -0.300 | -0.294 |
| 12.00 | -0.308 | -0.298 | -0.284 | -0.270 | -0.265 |
| 12.20 | -0.277 | -0.269 | -0.256 | -0.244 | -0.239 |
| 12.40 | -0.251 | -0.242 | -0.231 | -0.220 | -0.216 |
| 12.60 | -0.227 | -0.219 | -0.209 | -0.199 | -0.195 |
| 12.80 | -0.206 | -0.199 | -0.189 | -0.181 | -0.177 |
| 13.00 | -0.187 | -0.181 | -0.172 | -0.164 | -0.161 |
| 13.20 | -0.170 | -0.164 | -0.156 | -0.149 | -0.146 |
| 13.40 | -0.155 | -0.150 | -0.142 | -0.136 | -0.133 |
| 13.60 | -0.142 | -0.136 | -0.129 | -0.124 | -0.121 |
| 13.80 | -0.130 | -0.125 | -0.118 | -0.113 | -0.111 |
| 14.00 | -0.118 | -0.114 | -0.108 | -0.103 | -0.101 |
| 14.20 | -0.108 | -0.104 | -0.099 | -0.094 | -0.093 |
| 14.40 | -0.099 | -0.096 | -0.091 | -0.087 | -0.085 |
| 14.60 | -0.091 | -0.088 | -0.083 | -0.079 | -0.078 |
| 14.80 | -0.084 | -0.081 | -0.077 | -0.073 | -0.072 |
| 15.00 | -0.077 | -0.074 | -0.070 | -0.067 | -0.066 |
| 20.00 | -0.013 | -0.013 | -0.012 | -0.012 | -0.011 |
| 40.00 | 0.000 | 0.000 | 0.000 | 0.000 | 0.000 |

Table 6: The calculated interaction energy values (in $cm^{-1}$) for the *A1* excited state of the Sr-$H_2$ complex. The intermolecular distance values $R$ are given in angstroms

| $\theta =$ R | 0.00 | 25.8737249750682 | 47.3758416495282 | 68.7082259546949 | 90.00 |
|---|---|---|---|---|---|
| 4.20 | 659.313 | 732.150 | 819.941 | 881.057 | 902.528 |
| 4.40 | 440.905 | 519.873 | 600.215 | 657.478 | 678.039 |
| 4.60 | 280.350 | 393.925 | 436.163 | 482.976 | 500.679 |
| 4.80 | 165.321 | 205.247 | 330.734 | 351.508 | 364.320 |
| 5.00 | 85.017 | 126.207 | 184.662 | 263.554 | 261.567 |
| 5.20 | 30.563 | 71.675 | 122.357 | 168.746 | 185.374 |
| 5.40 | -5.043 | 36.434 | 79.079 | 114.951 | 129.675 |
| 5.60 | -27.160 | 16.251 | 49.656 | 77.968 | 89.505 |
| 5.80 | -39.806 | 7.713 | 30.636 | 52.046 | 60.913 |
| 6.00 | -45.958 | 7.873 | 19.181 | 34.218 | 40.826 |
| 6.20 | -47.816 | 13.140 | 12.990 | 22.226 | 26.895 |
| 6.40 | -46.972 | 19.476 | 10.258 | 14.346 | 17.363 |
| 6.60 | -44.532 | 23.951 | 9.419 | 9.313 | 10.935 |
| 6.80 | -41.238 | 25.696 | 9.493 | 6.207 | 6.676 |
| 7.00 | -37.570 | 25.434 | 9.753 | 4.361 | 3.914 |
| 7.20 | -33.832 | 24.124 | 9.936 | 3.289 | 2.173 |
| 7.40 | -30.214 | 22.449 | 9.992 | 2.804 | 1.117 |
| 7.60 | -26.823 | 20.841 | 9.901 | 2.107 | 0.513 |
| 7.80 | -23.717 | 19.384 | 9.746 | 1.717 | 0.199 |
| 8.00 | -20.917 | 17.773 | 9.399 | 2.563 | 0.066 |
| 8.20 | -18.422 | 16.967 | 9.272 | 2.391 | 0.040 |
| 8.40 | -16.218 | 15.774 | 9.060 | 2.288 | 0.074 |
| 8.60 | -14.282 | 14.682 | 8.522 | 2.747 | 0.135 |
| 8.80 | -12.589 | 13.639 | 7.997 | 2.638 | 0.205 |
| 9.00 | -11.112 | 12.617 | 7.858 | 2.520 | 0.272 |
| 9.20 | -9.825 | 11.611 | 7.278 | 2.467 | 0.332 |
| 9.40 | -8.705 | 10.634 | 6.694 | 2.319 | 0.381 |
| 9.60 | -7.729 | 9.959 | 6.122 | 2.166 | 0.420 |
| 9.80 | -6.878 | 9.075 | 5.579 | 2.016 | 0.448 |
| 10.00 | -6.135 | 8.284 | 5.083 | 1.873 | 0.467 |
| 10.20 | -5.486 | 7.599 | 4.646 | 1.744 | 0.478 |
| 10.40 | -4.917 | 7.023 | 4.273 | 1.631 | 0.482 |
| 10.60 | -4.417 | 6.549 | 3.964 | 1.534 | 0.480 |
| 10.80 | -3.977 | 6.167 | 3.716 | 1.454 | 0.473 |
| 11.00 | -3.589 | 5.858 | 3.516 | 1.386 | 0.463 |
| 11.20 | -3.246 | 5.602 | 3.354 | 1.328 | 0.451 |
| 11.40 | -2.942 | 5.379 | 3.218 | 1.277 | 0.436 |
| 11.60 | -2.672 | 5.171 | 3.095 | 1.228 | 0.419 |

*Table 6 continues on next page...*

*Table 6 continues...*

| $\theta =$ R | 0.00 | 25.8737249750682 | 47.3758416495282 | 68.7082259546949 | 90.00 |
|---|---|---|---|---|---|
| 11.80 | -2.431 | 4.964 | 2.975 | 1.180 | 0.402 |
| 12.00 | -2.217 | 4.746 | 2.853 | 1.131 | 0.384 |
| 12.20 | -2.025 | 4.512 | 2.723 | 1.078 | 0.367 |
| 12.40 | -1.854 | 4.260 | 2.583 | 1.023 | 0.349 |
| 12.60 | -1.699 | 3.992 | 2.434 | 0.965 | 0.332 |
| 12.80 | -1.560 | 3.712 | 2.278 | 0.905 | 0.315 |
| 13.00 | -1.435 | 3.426 | 2.116 | 0.844 | 0.299 |
| 13.20 | -1.322 | 3.140 | 1.953 | 0.783 | 0.284 |
| 13.40 | -1.219 | 2.859 | 1.792 | 0.723 | 0.269 |
| 13.60 | -1.126 | 2.590 | 1.636 | 0.666 | 0.255 |
| 13.80 | -1.042 | 2.336 | 1.487 | 0.612 | 0.241 |
| 14.00 | -0.965 | 2.101 | 1.349 | 0.561 | 0.229 |
| 14.20 | -0.894 | 1.887 | 1.222 | 0.515 | 0.217 |
| 14.40 | -0.830 | 1.696 | 1.108 | 0.474 | 0.205 |
| 14.60 | -0.771 | 1.528 | 1.007 | 0.436 | 0.194 |
| 14.80 | -0.717 | 1.382 | 0.919 | 0.404 | 0.184 |
| 15.00 | -0.668 | 1.258 | 0.844 | 0.376 | 0.174 |
| 20.00 | -0.149 | 0.515 | 0.330 | 0.134 | 0.049 |
| 40.00 | -0.004 | 0.026 | 0.014 | 0.005 | 0.002 |

Table 7: The calculated interaction energy values (in $cm^{-1}$) for the *B1* excited state of the Sr-$H_2$ complex. The intermolecular distance values $R$ are given in angstroms

| $\theta =$ R | 0.00 | 25.8737249750682 | 47.3758416495282 | 68.7082259546949 | 90.00 |
|---|---|---|---|---|---|
| 2.40 | | | 2252.769 | 1278.118 | 915.305 |
| 2.60 | | | 976.306 | 375.871 | 151.870 |
| 2.80 | | 861.964 | 404.481 | 19.284 | -125.565 |
| 3.00 | | 455.558 | 152.928 | -105.837 | -204.401 |
| 3.20 | | 249.434 | 39.873 | -141.684 | -211.547 |
| 3.40 | | 136.882 | -14.230 | -146.502 | -197.762 |
| 3.60 | 134.317 | 70.688 | -41.810 | -141.195 | -180.004 |
| 3.80 | 78.441 | 30.213 | -55.646 | -132.235 | -162.356 |
| 4.00 | 42.967 | 5.739 | -61.142 | -121.332 | -145.115 |
| 4.20 | 21.030 | -8.210 | -61.145 | -109.113 | -128.113 |
| 4.40 | 8.172 | -15.196 | -57.592 | -96.250 | -111.592 |
| 4.60 | 1.290 | -17.679 | -51.999 | -83.485 | -96.005 |
| 4.80 | -1.860 | -17.435 | -45.518 | -71.417 | -81.733 |
| 5.00 | -2.846 | -15.715 | -38.932 | -60.420 | -68.996 |
| 5.20 | -2.681 | -13.343 | -32.716 | -50.683 | -57.867 |
| 5.40 | -1.988 | -10.827 | -27.123 | -42.252 | -48.308 |
| 5.60 | -1.117 | -8.451 | -22.258 | -35.075 | -40.206 |
| 5.80 | -0.230 | -6.355 | -18.127 | -29.038 | -33.405 |
| 6.00 | 0.600 | -4.590 | -14.676 | -24.006 | -27.739 |
| 6.20 | 1.321 | -3.157 | -11.832 | -19.842 | -23.049 |
| 6.40 | 1.884 | -2.028 | -9.513 | -16.420 | -19.185 |
| 6.60 | 2.275 | -1.161 | -7.642 | -13.619 | -16.013 |
| 6.80 | 2.506 | -0.512 | -6.142 | -11.334 | -13.414 |
| 7.00 | 2.611 | -0.038 | -4.944 | -9.469 | -11.282 |
| 7.20 | 2.625 | 0.302 | -3.988 | -7.946 | -9.532 |
| 7.40 | 2.578 | 0.537 | -3.226 | -6.699 | -8.090 |
| 7.60 | 2.490 | 0.695 | -2.616 | -5.673 | -6.898 |
| 7.80 | 2.378 | 0.794 | -2.127 | -4.826 | -5.907 |
| 8.00 | 2.252 | 0.850 | -1.735 | -4.123 | -5.081 |
| 8.20 | 2.119 | 0.875 | -1.418 | -3.538 | -4.388 |
| 8.40 | 1.985 | 0.878 | -1.161 | -3.047 | -3.804 |
| 8.60 | 1.853 | 0.865 | -0.953 | -2.635 | -3.310 |
| 8.80 | 1.726 | 0.841 | -0.783 | -2.287 | -2.892 |
| 9.00 | 1.604 | 0.811 | -0.645 | -1.993 | -2.535 |
| 9.20 | 1.488 | 0.776 | -0.531 | -1.743 | -2.230 |
| 9.40 | 1.380 | 0.738 | -0.438 | -1.529 | -1.968 |
| 9.60 | 1.278 | 0.700 | -0.362 | -1.346 | -1.742 |
| 9.80 | 1.183 | 0.661 | -0.298 | -1.189 | -1.547 |

*Table 7 continues on next page...*

*Table 7 continues...*

| $\theta =$ R | 0.00 | 25.8737249750682 | 47.3758416495282 | 68.7082259546949 | 90.00 |
|---|---|---|---|---|---|
| 10.00 | 1.096 | 0.623 | -0.246 | -1.052 | -1.376 |
| 10.20 | 1.014 | 0.586 | -0.202 | -0.933 | -1.227 |
| 10.40 | 0.939 | 0.550 | -0.166 | -0.830 | -1.097 |
| 10.60 | 0.870 | 0.516 | -0.135 | -0.740 | -0.983 |
| 10.80 | 0.807 | 0.484 | -0.110 | -0.661 | -0.883 |
| 11.00 | 0.748 | 0.454 | -0.089 | -0.592 | -0.794 |
| 11.20 | 0.695 | 0.425 | -0.071 | -0.531 | -0.717 |
| 11.40 | 0.645 | 0.399 | -0.056 | -0.478 | -0.648 |
| 11.60 | 0.599 | 0.374 | -0.044 | -0.431 | -0.587 |
| 11.80 | 0.557 | 0.350 | -0.034 | -0.390 | -0.533 |
| 12.00 | 0.519 | 0.328 | -0.026 | -0.353 | -0.485 |
| 12.20 | 0.483 | 0.307 | -0.018 | -0.320 | -0.442 |
| 12.40 | 0.450 | 0.288 | -0.012 | -0.291 | -0.403 |
| 12.60 | 0.419 | 0.270 | -0.008 | -0.265 | -0.369 |
| 12.80 | 0.391 | 0.253 | -0.003 | -0.242 | -0.338 |
| 13.00 | 0.365 | 0.237 | 0.000 | -0.221 | -0.309 |
| 13.20 | 0.341 | 0.223 | 0.003 | -0.202 | -0.284 |
| 13.40 | 0.319 | 0.209 | 0.005 | -0.185 | -0.261 |
| 13.60 | 0.298 | 0.197 | 0.007 | -0.169 | -0.240 |
| 13.80 | 0.279 | 0.185 | 0.009 | -0.155 | -0.221 |
| 14.00 | 0.262 | 0.174 | 0.010 | -0.143 | -0.204 |
| 14.20 | 0.246 | 0.164 | 0.011 | -0.131 | -0.189 |
| 14.40 | 0.231 | 0.154 | 0.012 | -0.121 | -0.175 |
| 14.60 | 0.217 | 0.145 | 0.012 | -0.112 | -0.162 |
| 14.80 | 0.204 | 0.137 | 0.013 | -0.103 | -0.150 |
| 15.00 | 0.192 | 0.130 | 0.013 | -0.095 | -0.139 |
| 20.00 | 0.051 | 0.036 | 0.008 | -0.018 | -0.029 |
| 40.00 | 0.002 | 0.001 | 0.000 | 0.000 | -0.001 |

Table 8: The calculated interaction energy values (in $cm^{-1}$) for the *B2* excited state of the Sr-$H_2$ complex. The intermolecular distance values $R$ are given in angstroms

| $\theta =$ R | 0.00 | 25.8737249750682 | 47.3758416495282 | 68.7082259546949 | 90.00 |
|---|---|---|---|---|---|
| 1.80 | | | | 9274.936 | |
| 2.00 | | | | 2266.045 | |
| 2.10 | | | | | -719.305 |
| 2.15 | | | | | -1204.027 |
| 2.20 | | | 2149.760 | -572.880 | -1553.771 |
| 2.25 | | | | | -1793.648 |
| 2.30 | | | | | -1944.812 |
| 2.35 | | | | | -2026.257 |
| 2.40 | | 2670.659 | 377.700 | -1408.451 | -2052.789 |
| 2.60 | | 1218.061 | -254.893 | -1418.265 | -1838.565 |
| 2.80 | | 547.039 | -409.899 | -1170.687 | -1445.894 |
| 3.00 | | 241.384 | -395.362 | -900.531 | -1083.355 |
| 3.20 | | 98.373 | -338.532 | -681.214 | -804.803 |
| 3.40 | | 26.424 | -282.881 | -520.868 | -605.969 |
| 3.60 | 134.317 | -12.975 | -238.118 | -407.233 | -467.125 |
| 3.80 | 78.441 | -35.355 | -203.128 | -325.850 | -368.843 |
| 4.00 | 42.967 | -47.542 | -174.938 | -265.394 | -296.661 |
| 4.20 | 21.030 | -53.352 | -151.329 | -218.518 | -241.349 |
| 4.40 | 8.172 | -55.439 | -131.238 | -180.988 | -197.558 |
| 4.60 | 1.290 | -55.865 | -114.301 | -150.423 | -162.209 |
| 4.80 | -1.860 | -54.737 | -100.329 | -125.371 | -133.389 |
| 5.00 | -2.846 | -56.974 | -89.166 | -104.549 | -109.791 |
| 5.20 | -2.681 | -60.762 | -80.502 | -87.836 | -90.452 |
| 5.40 | -1.988 | -66.074 | -73.846 | -74.209 | -74.615 |
| 5.60 | -1.117 | -72.147 | -68.524 | -63.041 | -61.659 |
| 5.80 | -0.230 | -78.563 | -63.919 | -53.817 | -51.066 |
| 6.00 | 0.600 | -84.389 | -59.624 | -46.099 | -42.409 |
| 6.20 | 1.321 | -87.385 | -55.450 | -39.599 | -35.334 |
| 6.40 | 1.884 | -85.683 | -51.377 | -34.116 | -29.550 |
| 6.60 | 2.275 | -80.097 | -47.407 | -29.484 | -24.818 |
| 6.80 | 2.506 | -72.573 | -43.573 | -25.578 | -20.940 |
| 7.00 | 2.611 | -64.765 | -39.902 | -22.272 | -17.751 |
| 7.20 | 2.625 | -57.477 | -36.400 | -19.540 | -15.121 |
| 7.40 | 2.578 | -51.007 | -33.128 | -17.208 | -12.941 |
| 7.60 | 2.490 | -45.405 | -30.128 | -14.878 | -11.127 |
| 7.80 | 2.378 | -40.606 | -27.408 | -13.571 | -9.609 |
| 8.00 | 2.252 | -36.495 | -24.969 | -11.897 | -8.334 |
| 8.20 | 2.119 | -32.839 | -22.777 | -10.900 | -7.256 |

*Table 8 continues on next page...*

*Table 8 continues...*

| θ = R | 0.00 | 25.8737249750682 | 47.3758416495282 | 68.7082259546949 | 90.00 |
|---|---|---|---|---|---|
| 8.40 | 1.985 | -29.808 | -20.518 | -9.660 | -6.341 |
| 8.60 | 1.853 | -27.017 | -18.984 | -8.586 | -5.563 |
| 8.80 | 1.726 | -24.438 | -17.145 | -7.645 | -4.896 |
| 9.00 | 1.604 | -22.077 | -15.460 | -6.812 | -4.325 |
| 9.20 | 1.488 | -19.904 | -13.906 | -6.070 | -3.832 |
| 9.40 | 1.380 | -17.914 | -12.474 | -5.409 | -3.406 |
| 9.60 | 1.278 | -16.108 | -11.562 | -4.821 | -3.035 |
| 9.80 | 1.183 | -14.491 | -10.345 | -4.301 | -2.712 |
| 10.00 | 1.096 | -13.067 | -9.267 | -3.846 | -2.429 |
| 10.20 | 1.014 | -11.835 | -8.330 | -3.449 | -2.181 |
| 10.40 | 0.939 | -10.787 | -7.531 | -3.107 | -1.962 |
| 10.60 | 0.870 | -9.905 | -6.860 | -2.812 | -1.769 |
| 10.80 | 0.807 | -9.169 | -6.301 | -2.560 | -1.598 |
| 11.00 | 0.748 | -8.552 | -5.837 | -2.343 | -1.447 |
| 11.20 | 0.695 | -8.028 | -5.447 | -2.156 | -1.313 |
| 11.40 | 0.645 | -7.570 | -5.114 | -1.991 | -1.193 |
| 11.60 | 0.599 | -7.154 | -4.819 | -1.845 | -1.087 |
| 11.80 | 0.557 | -6.763 | -4.547 | -1.713 | -0.992 |
| 12.00 | 0.519 | -6.381 | -4.288 | -1.591 | -0.907 |
| 12.20 | 0.483 | -6.000 | -4.034 | -1.477 | -0.830 |
| 12.40 | 0.450 | -5.616 | -3.782 | -1.369 | -0.761 |
| 12.60 | 0.419 | -5.229 | -3.529 | -1.267 | -0.699 |
| 12.80 | 0.391 | -4.841 | -3.276 | -1.170 | -0.643 |
| 13.00 | 0.365 | -4.457 | -3.027 | -1.079 | -0.592 |
| 13.20 | 0.341 | -4.082 | -2.783 | -0.991 | -0.546 |
| 13.40 | 0.319 | -3.721 | -2.547 | -0.911 | -0.504 |
| 13.60 | 0.298 | -3.378 | -2.323 | -0.835 | -0.466 |
| 13.80 | 0.279 | -3.058 | -2.112 | -0.765 | -0.431 |
| 14.00 | 0.262 | -2.763 | -1.918 | -0.701 | -0.399 |
| 14.20 | 0.246 | -2.495 | -1.741 | -0.642 | -0.370 |
| 14.40 | 0.231 | -2.254 | -1.581 | -0.590 | -0.344 |
| 14.60 | 0.217 | -2.042 | -1.440 | -0.543 | -0.319 |
| 14.80 | 0.204 | -1.857 | -1.316 | -0.501 | -0.297 |
| 15.00 | 0.192 | -1.697 | -1.208 | -0.465 | -0.277 |
| 20.00 | 0.051 | -0.610 | -0.416 | -0.134 | -0.061 |
| 40.00 | 0.002 | -0.029 | -0.017 | -0.004 | -0.002 |

Table 9: The calculated interaction energy values (in $cm^{-1}$) for the ground state of the Yb-$H_2$ complex. The intermolecular distance values $R$ are given in angstroms

| $\theta =$ R | 0.00 | 25.8737249750682 | 47.3758416495282 | 68.7082259546949 | 90.00 |
|---|---|---|---|---|---|
| 4.00 | 125.427 | 127.836 | 132.270 | 136.533 | 138.255 |
| 4.20 | 52.085 | 55.365 | 61.153 | 66.329 | 68.362 |
| 4.40 | 8.729 | 12.144 | 18.138 | 23.373 | 25.406 |
| 4.60 | -15.204 | -12.002 | -6.375 | -1.518 | 0.351 |
| 4.80 | -26.920 | -24.092 | -19.095 | -14.809 | -13.159 |
| 5.00 | -31.270 | -28.841 | -24.573 | -20.918 | -19.504 |
| 5.20 | -31.406 | -29.375 | -25.801 | -22.744 | -21.567 |
| 5.40 | -29.315 | -27.635 | -24.699 | -22.178 | -21.214 |
| 5.60 | -26.215 | -24.845 | -22.453 | -20.397 | -19.604 |
| 5.80 | -22.821 | -21.711 | -19.780 | -18.107 | -17.460 |
| 6.00 | -19.523 | -18.629 | -17.063 | -15.720 | -15.191 |
| 6.20 | -16.518 | -15.794 | -14.547 | -13.445 | -13.022 |
| 6.40 | -13.877 | -13.308 | -12.287 | -11.394 | -11.064 |
| 6.60 | -11.611 | -11.155 | -10.337 | -9.608 | -9.339 |
| 6.80 | -9.701 | -9.323 | -8.674 | -8.077 | -7.850 |
| 7.00 | -8.105 | -7.810 | -7.262 | -6.784 | -6.598 |
| 7.40 | -5.687 | -5.480 | -5.120 | -4.797 | -4.673 |
| 7.80 | -4.029 | -3.894 | -3.646 | -3.422 | -3.342 |
| 8.20 | -2.905 | -2.806 | -2.627 | -2.476 | -2.418 |
| 8.60 | -2.104 | -2.053 | -1.929 | -1.817 | -1.773 |
| 9.00 | -1.578 | -1.522 | -1.431 | -1.363 | -1.318 |
| 9.40 | -1.186 | -1.148 | -1.076 | -1.021 | -0.988 |
| 9.80 | -0.895 | -0.867 | -0.827 | -0.789 | -0.762 |
| 10.20 | -0.701 | -0.679 | -0.638 | -0.602 | -0.599 |
| 10.60 | -0.547 | -0.531 | -0.507 | -0.473 | -0.455 |

Table 10: The calculated interaction energy values (in $cm^{-1}$) for the *A1* excited state of the Yb-$H_2$ complex. The intermolecular distance values $R$ are given in angstroms

| $\theta =$ R | 0.00 | 25.8737249750682 | 47.3758416495282 | 68.7082259546949 | 90.00 |
|---|---|---|---|---|---|
| 3.60 | | | | 1689.289 | |
| 3.80 | | 1137.391 | 1237.004 | 1311.578 | |
| 4.00 | 753.881 | 813.168 | 915.398 | 993.358 | 1028.672 |
| 4.20 | 508.188 | 565.573 | 662.329 | 736.788 | 771.189 |
| 4.40 | 327.429 | 382.394 | 469.229 | 536.854 | 568.735 |
| 4.60 | 197.565 | 202.564 | 326.062 | 384.846 | 413.525 |
| 4.80 | 106.559 | 138.766 | 200.623 | 271.793 | 296.824 |
| 5.00 | 44.535 | 77.149 | 131.739 | 164.770 | 210.453 |
| 5.20 | 3.690 | 35.090 | 84.367 | 125.027 | 147.407 |
| 5.40 | -21.980 | 8.686 | 49.810 | 83.563 | 101.960 |
| 5.60 | -37.009 | -3.033 | 26.675 | 54.050 | 69.591 |
| 5.80 | -44.749 | -11.623 | 11.938 | 33.661 | 46.804 |
| 6.00 | -47.637 | -11.832 | 3.136 | 19.901 | 30.954 |
| 6.20 | -47.412 | -9.287 | -1.632 | 10.828 | 20.070 |
| 6.40 | -45.293 | -6.174 | -3.794 | 5.194 | 12.700 |
| 6.60 | -42.116 | -3.599 | -4.417 | 1.611 | 7.793 |
| 6.80 | -38.442 | -1.799 | -4.207 | -0.607 | 4.592 |
| 7.00 | -34.636 | -0.345 | -3.382 | -1.674 | 2.561 |
| 7.40 | -27.422 | 0.667 | -1.592 | -2.013 | 0.591 |
| 7.80 | -21.328 | 0.911 | -0.940 | -1.723 | 0.023 |
| 8.20 | -16.483 | 1.100 | -0.609 | -1.155 | -0.007 |
| 8.60 | -12.750 | 1.019 | -0.198 | -0.559 | 0.121 |
| 9.00 | -9.913 | 0.923 | -0.032 | -0.258 | 0.259 |
| 9.40 | -7.768 | 0.829 | 0.074 | -0.070 | 0.360 |
| 9.80 | -6.142 | 0.632 | 0.138 | 0.070 | 0.416 |
| 10.20 | -4.903 | 0.490 | 0.192 | 0.134 | 0.436 |
| 10.60 | -3.951 | 0.353 | 0.193 | 0.168 | 0.428 |

Table 11: The calculated interaction energy values (in $cm^{-1}$) for the *B1* excited state of the Yb-$H_2$ complex. The intermolecular distance values $R$ are given in angstroms

| $\theta =$ R | 0.00 | 25.8737249750682 | 47.3758416495282 | 68.7082259546949 | 90.00 |
|---|---|---|---|---|---|
| 2.20 | | | | 2035.239 | 1541.443 |
| 2.40 | | | | 630.008 | 338.893 |
| 2.60 | | | 537.004 | 56.310 | -123.283 |
| 2.80 | 736.654 | 521.403 | 154.802 | -154.853 | -271.808 |
| 3.00 | 379.891 | 237.521 | -7.802 | -218.844 | -299.460 |
| 3.20 | 197.576 | 97.693 | -75.503 | -226.561 | -284.951 |
| 3.40 | 99.163 | 26.152 | -101.372 | -213.603 | -257.432 |
| 3.60 | 43.924 | -10.762 | -107.502 | -193.289 | -226.971 |
| 3.80 | 13.292 | -28.696 | -103.656 | -170.572 | -196.913 |
| 4.00 | -2.642 | -35.541 | -94.622 | -147.687 | -168.614 |
| 4.20 | -9.803 | -35.993 | -83.224 | -125.840 | -142.674 |
| 4.40 | -11.954 | -33.064 | -71.214 | -105.762 | -119.431 |
| 4.60 | -11.373 | -28.557 | -59.647 | -87.892 | -99.090 |
| 4.80 | -9.475 | -23.588 | -49.141 | -72.422 | -81.667 |
| 5.00 | -7.145 | -18.820 | -39.984 | -59.319 | -67.013 |
| 5.20 | -4.862 | -14.585 | -32.238 | -48.408 | -54.854 |
| 5.40 | -2.855 | -11.007 | -25.827 | -39.436 | -44.871 |
| 5.60 | -1.212 | -8.090 | -20.608 | -32.124 | -36.728 |
| 5.80 | 0.061 | -5.776 | -16.408 | -26.199 | -30.120 |
| 6.00 | 0.991 | -3.981 | -13.056 | -21.417 | -24.767 |
| 6.20 | 1.645 | -2.613 | -10.396 | -17.563 | -20.435 |
| 6.40 | 2.075 | -1.587 | -8.289 | -14.456 | -16.930 |
| 6.60 | 2.333 | -0.831 | -6.624 | -11.953 | -14.089 |
| 6.80 | 2.464 | -0.282 | -5.304 | -9.928 | -11.781 |
| 7.00 | 2.498 | 0.109 | -4.264 | -8.287 | -9.899 |
| 7.40 | 2.393 | 0.567 | -2.779 | -5.860 | -7.091 |
| 7.80 | 2.172 | 0.757 | -1.835 | -4.225 | -5.182 |
| 8.20 | 1.915 | 0.807 | -1.228 | -3.103 | -3.843 |
| 8.60 | 1.662 | 0.783 | -0.829 | -2.318 | -2.914 |
| 9.00 | 1.438 | 0.727 | -0.564 | -1.758 | -2.236 |
| 9.40 | 1.225 | 0.658 | -0.385 | -1.351 | -1.732 |
| 9.80 | 1.049 | 0.586 | -0.264 | -1.047 | -1.367 |
| 10.20 | 0.898 | 0.517 | -0.179 | -0.827 | -1.087 |
| 10.60 | 0.770 | 0.458 | -0.121 | -0.652 | -0.872 |

Table 12: The calculated interaction energy values (in $cm^{-1}$) for the *B2* excited state of the Yb-$H_2$ complex. The intermolecular distance values $R$ are given in angstroms

| $\theta =$ R | 0.00 | 25.8737249750682 | 47.3758416495282 | 68.7082259546949 | 90.00 |
|---|---|---|---|---|---|
| 1.80 | | | 11148.069 | | 3106.143 |
| 2.00 | | | 4084.881 | 363.171 | -967.024 |
| 2.20 | | | 1030.428 | -1331.063 | -2176.307 |
| 2.40 | | | -131.772 | -1632.713 | -2174.594 |
| 2.60 | | 726.841 | -480.367 | -1438.909 | -1788.686 |
| 2.80 | 736.654 | 261.955 | -521.018 | -1141.957 | -1371.947 |
| 3.00 | 379.891 | 60.529 | -465.004 | -877.985 | -1034.682 |
| 3.20 | 197.576 | -25.119 | -391.192 | -674.327 | -786.007 |
| 3.40 | 99.163 | -60.068 | -323.588 | -523.323 | -606.515 |
| 3.60 | 43.924 | -71.867 | -266.719 | -411.239 | -475.445 |
| 3.80 | 13.292 | -72.673 | -219.826 | -326.336 | -377.247 |
| 4.00 | -2.642 | -67.728 | -180.208 | -260.493 | -301.784 |
| 4.20 | -9.803 | -60.380 | -147.829 | -208.453 | -242.578 |
| 4.40 | -11.954 | -52.182 | -120.837 | -166.858 | -195.476 |
| 4.60 | -11.373 | -44.264 | -98.525 | -133.508 | -157.763 |
| 4.80 | -9.475 | -37.389 | -80.357 | -106.815 | -127.518 |
| 5.00 | -7.145 | -32.036 | -65.795 | -85.516 | -103.273 |
| 5.20 | -4.862 | -28.552 | -54.279 | -68.579 | -83.854 |
| 5.40 | -2.855 | -26.736 | -45.618 | -55.159 | -68.307 |
| 5.60 | -1.212 | -26.818 | -38.797 | -44.564 | -55.856 |
| 5.80 | 0.061 | -28.717 | -33.681 | -36.215 | -45.876 |
| 6.00 | 0.991 | -31.738 | -29.722 | -29.635 | -37.858 |
| 6.20 | 1.645 | -34.265 | -26.718 | -24.436 | -31.402 |
| 6.40 | 2.075 | -34.957 | -24.355 | -20.309 | -26.182 |
| 6.60 | 2.333 | -33.868 | -22.370 | -19.011 | -21.952 |
| 6.80 | 2.464 | -31.682 | -20.568 | -16.169 | -18.503 |
| 7.00 | 2.498 | -28.982 | -18.834 | -13.875 | -15.679 |
| 7.40 | 2.393 | -23.301 | -15.464 | -10.416 | -11.429 |
| 7.80 | 2.172 | -18.270 | -12.371 | -7.966 | -8.494 |
| 8.20 | 1.915 | -14.179 | -9.738 | -6.157 | -6.422 |
| 8.60 | 1.662 | -10.980 | -7.474 | -4.785 | -4.930 |
| 9.00 | 1.438 | -8.558 | -5.784 | -3.733 | -3.838 |
| 9.40 | 1.225 | -6.701 | -4.508 | -2.921 | -3.024 |
| 9.80 | 1.049 | -5.292 | -3.548 | -2.321 | -2.404 |
| 10.20 | 0.898 | -4.218 | -2.822 | -1.959 | -1.934 |
| 10.60 | 0.770 | -3.394 | -2.267 | -1.575 | -1.575 |

Table 13: The calculated interaction energy values (in $cm^{-1}$) for the ground and excited states of the Sr-He complex. The intermolecular distance values $R$ are given in angstroms

| R | Ground State | *A1* | *B1* |
|---|---|---|---|
| 2.00 | 8088.471 | 7064.756 | 4669.226 |
| 2.20 | 5270.747 | 4819.656 | 2259.339 |
| 2.40 | 3752.630 | 3842.089 | 1223.770 |
| 2.60 | 2786.456 | 3342.138 | 751.645 |
| 2.80 | 2079.498 | 2991.507 | 502.063 |
| 3.00 | 1530.017 | 2661.554 | 344.365 |
| 3.20 | 1102.125 | 2308.921 | 232.694 |
| 3.40 | 776.213 | 1934.880 | 150.958 |
| 3.60 | 534.743 | 1564.176 | 92.026 |
| 3.80 | 360.551 | 1225.624 | 51.119 |
| 4.00 | 237.880 | 937.082 | 24.079 |
| 4.20 | 153.351 | 702.922 | 7.212 |
| 4.40 | 96.286 | 519.288 | -2.575 |
| 4.60 | 58.494 | 378.848 | -7.720 |
| 4.80 | 33.929 | 273.362 | -9.987 |
| 5.00 | 18.299 | 195.180 | -10.539 |
| 5.20 | 8.625 | 137.886 | -10.116 |
| 5.40 | 2.855 | 96.340 | -9.192 |
| 5.60 | -0.412 | 66.520 | -8.064 |
| 5.80 | -2.118 | 45.320 | -6.915 |
| 6.00 | -2.885 | 30.385 | -5.847 |
| 6.20 | -3.109 | 19.956 | -4.905 |
| 6.40 | -3.037 | 12.742 | -4.101 |
| 6.60 | -2.816 | 7.809 | -3.427 |
| 6.80 | -2.531 | 4.481 | -2.867 |
| 7.00 | -2.233 | 2.275 | -2.404 |
| 7.40 | -1.683 | -0.050 | -1.706 |
| 7.80 | -1.247 | -0.882 | -1.229 |
| 8.20 | -0.921 | -1.060 | -0.899 |
| 8.60 | -0.683 | -0.979 | -0.666 |
| 9.00 | -0.510 | -0.818 | -0.499 |
| 9.40 | -0.384 | -0.653 | -0.378 |
| 9.80 | -0.292 | -0.511 | -0.290 |
| 10.20 | -0.226 | -0.396 | -0.226 |
| 10.60 | -0.177 | -0.308 | -0.178 |

Table 14: The calculated interaction energy values (in $cm^{-1}$) for the ground and excited states of the Yb-He complex. The intermolecular distance values $R$ are given in angstroms

| R | Ground State | *A1* | *B1* |
|---|---|---|---|
| 2.00 | | 6676.506 | 3597.061 |
| 2.20 | | 5059.813 | 1837.823 |
| 2.40 | | 4257.211 | 1047.476 |
| 2.60 | | 3718.356 | 645.499 |
| 2.80 | | 3238.512 | 408.110 |
| 3.00 | | 2756.522 | 252.938 |
| 3.20 | | 2274.590 | 148.374 |
| 3.40 | | 1818.680 | 78.977 |
| 3.60 | | 1414.566 | 34.764 |
| 3.80 | | 1076.049 | 8.243 |
| 4.00 | 141.799 | 804.346 | -6.452 |
| 4.20 | 84.430 | 592.860 | -13.651 |
| 4.40 | 48.049 | 431.861 | -16.317 |
| 4.60 | 25.520 | 311.319 | -16.399 |
| 4.80 | 11.950 | 222.231 | -15.157 |
| 5.00 | 4.046 | 157.083 | -13.364 |
| 5.20 | -0.344 | 109.886 | -11.460 |
| 5.40 | -2.602 | 75.999 | -9.661 |
| 5.60 | -3.592 | 51.879 | -8.060 |
| 5.80 | -3.864 | 34.868 | -6.684 |
| 6.00 | -3.743 | 22.984 | -5.525 |
| 6.20 | -3.432 | 14.767 | -4.563 |
| 6.40 | -3.048 | 9.150 | -3.774 |
| 6.60 | -2.652 | 5.362 | -3.125 |
| 6.80 | -2.282 | 2.858 | -2.599 |
| 7.00 | -1.947 | 1.220 | -2.183 |
| 7.40 | -1.406 | -0.428 | -1.529 |
| 7.80 | -1.016 | -0.953 | -1.097 |
| 8.20 | -0.779 | -1.010 | -0.799 |
| 8.60 | -0.544 | -0.895 | -0.591 |
| 9.00 | -0.412 | -0.737 | -0.443 |
| 9.40 | -0.311 | -0.586 | -0.346 |
| 9.80 | -0.236 | -0.449 | -0.258 |
| 10.20 | -0.180 | -0.348 | -0.209 |
| 10.60 | -0.140 | -0.277 | -0.154 |

# References

[1] R. Bukowski, J. Sadlej, B. Jeziorski, P. Jankowski, K. Szalewicz, S. A. Kucharski, H. L. Williams, and B. M. Rice, *J. Chem. Phys.* **110**, 3785 (1999).

[2] R. R. Toczyłowski and S. M. Cybulski, *J. Chem. Phys.* **112**, 4604 (2000).

[3] T. B. Pedersen, J. López Cacheiro, B. Fernández, and H. Koch, *J. Chem. Phys.* **117**, 6562 (2002).

[4] K. T. Tang and J. P. Toennies, *J. Chem. Phys.* **80**, 3726 (1984).
